# Supplementary material for: Real-Time Face and Landmark Localization for Eyeblink Detection
Source: arXiv:2006.00816 source file (2020-07-15)
Supplement: Supplementary file 1 [file appendixA.tex]

\chapter{Appendix}
\newpage

\section{False negatives}
\label{appendix:falsenegatives}
\begin{figure}[H]
\centering
\includegraphics[width=\textwidth,height=.9\textheight,keepaspectratio]{figures/appendix/haarfalseneg.png}
\caption{96 faces in the AFLW database that the Haar facedetector failed to identify}
\label{fig:haarfalseneg}
\end{figure}

\begin{figure}[H]
\centering
\includegraphics[width=\textwidth,height=.9\textheight,keepaspectratio]{figures/appendix/hogfalseneg.png}
\caption{96 faces in the AFLW database that the HOG facedetector failed to identify}
\label{fig:hogfalseneg}
\end{figure}

\begin{figure}[H]
\centering
\includegraphics[width=\textwidth,height=.9\textheight,keepaspectratio]{figures/appendix/cnnfalseneg.png}
\caption{96 faces in the AFLW database that the CNN facedetector failed to identify}
\label{fig:cnnfalseneg}
\end{figure}

\section{False positives}
\label{appendix:falsepositives}

\begin{figure}[H]
\centering
\includegraphics[width=\textwidth,height=.88\textheight,keepaspectratio]{figures/appendix/haarfalsepos.png}
\caption{96 images that where classified as face by the Haar face detector but not annotated in the AFLW database}
\label{fig:haarfalsepos}
\end{figure}

\begin{figure}[H]
\centering
\includegraphics[width=\textwidth,height=.9\textheight,keepaspectratio]{figures/appendix/hogfalsepos.png}
\caption{96 images that where classified as face by the HOG face detector but not annotated in the AFLW database}
\label{fig:hogfalsepos}
\end{figure}

\begin{figure}[H]
\centering
\includegraphics[width=\textwidth,height=.9\textheight,keepaspectratio]{figures/appendix/cnnfalsepos.png}
\caption{96 images that where classified as face by the CNN face detector but not annotated in the AFLW database}
\label{fig:cnnfalsepos}
\end{figure}

\section{NVIDIA Titan X (Pascal) block diagram}
\label{appendix:titanxchiplayout}

\begin{figure}[H]
\centering
\includegraphics[width=\textwidth,height=.85\textheight,keepaspectratio]{figures/appendix/titanxchiplayout.png}
\caption{NVIDIA Titan X (Pascal) chip block diagram. The GPU is based on the NVIDIA GP102 die with 2 SMs disabled. This leaves 28 SMs with 128 CUDA cores each, resulting in a total of 3584 CUDA cores.}% Image from https://www.gamersnexus.net/images/media/2016/gpu/titan-xp/titan-xpascal-gp102-block-diagram.png}}
\label{fig:titanxchiplayout}
\end{figure}

\section{Multiple stream NVVP output}
\label{appendix:NNVPstream}

\begin{figure}[H]
\centering
\includegraphics[width=\textwidth,height=.83\textheight,keepaspectratio]{figures/appendix/nvvpstreamssmallerrotated.png}
\caption{Output of the NVIDIA Visual Profiler for the face detection implementation with seperate streams for each image scale. The multiple lanes in the 'compute' row indicate concurrent kernel execution, which only happens for the larger \texttt{gradientHistogram} and \texttt{classifier} kernels.}
\label{fig:NNVPstream}
\end{figure}

\section{Multiple stream NVVP output for multi image implementation}
\label{appendix:combinefinal}

\begin{figure}[H]
\centering
\includegraphics[width=\textwidth,height=.9\textheight,keepaspectratio]{figures/appendix/nvvpstreamcombineimage.png}
\caption{Output of the NVIDIA Visual Profiler for the face detection implementation where the GPU is running face detection on batches of 16 images. Each image scale has its own GPU stream. The multiple lanes in the 'compute' row indicate concurrent kernel execution, which happens for the kernels that are too small to occupy all GPU SMs on their own.}
\label{NVVPstreammultipleimage}
\end{figure}
