# Supplementary material for: Real-Time Face and Landmark Localization for Eyeblink Detection
Source: arXiv:2006.00816 source file (2020-07-15)
Supplement: Supplementary file 2 [file dictionary.tex]

\chapter*{List of definitions}

\begin{description}
\item[Warp]  Group of 32 threads on a GPU
\end{description}
